# Supplementary material for: Inertial movements of the iris as the origin of post-saccadic oscillations
Source: arXiv:1709.00016 source file (2018-04-10)
Supplement: Supplementary file 1 [file bouzat-PhyRevLett2018-SupMat.pdf]

# Supplemental Material to “Inertial movements of the iris as the origin of post saccadic oscillations”

S. Bouzat[1*], M. L. Freije[2], A. L. Frapiccini[2], G. Gasaneo[2]
[1]*Consejo Nacional de Investigaciones Científicas y Técnicas, Centro Atómico Bariloche (CNEA), (8400) Bariloche, Río Negro, Argentina.*
[2]*Neufisur - Departamento de Física, Universidad Nacional del Sur - IFISUR, Bahía Blanca (8000), Buenos Aires, Argentina.**

We analyze the relation between the pupil and pupil minus corneal reflection (p-CR) signals in the p-CR eye trackers used in the experiments in [1, 2]. We show that the qualitative results obtained with our model when modeling the pupil motion (in particular the dependence of the PSO oscillations on the saccade size) are also expected to be representative of the results obtained with the p-CR eye trackers.

## APPROXIMATION FOR P-CR SIGNAL.

Pupil based video eye-trackers use the pupil position in their camera image to determine gaze position. This technique requires the head to be very still. In contrast, in p-CR eye trackers the pupil centre and the centre of the corneal reflection are subtracted from each other to produce a gaze signal which compensates the motion of the head. However, in [2] it was shown that some p-CR eye trackers may overestimate the amplitude of the PSO oscillations.

Here we develop an approximation for the gaze signal obtained from p-CR eye trackers. For this we follow the arguments and findings in Ref. [2].

Let us call $p(t)$ and $c(t)$ the pupil and corneal reflexion signals, respectively, measured in camera pixels.

For the pupil displacement we can write

$$p(t) - p_0 = x(t) + y(t). \tag{1}$$

Here $p_0 = p(0)$ is the initial value, $x(t)$ is the displacement of the eyeball which is assumed to grow monotonously from $x(0) = 0$ to $x_m = x(t \to \infty)$ (the saccade size). Meanwhile $y(t)$ is the relative position of the pupil satisfying $y(0) = y(t \to \infty) = 0$. Here $t \to \infty$ means the long time limit which is achieved when the saccade is ended and the PSO suppressed. The functions $x(t)$ and $y(t)$ can be thought as the dynamical variables defined in the main text, but the developments presented here are independent of the considerations of the model, and only require the above mentioned initial and long time conditions to hold, and $x(t)$ to be monotonous.

The corneal reflection signal displacement (in camera pixels) can be written as

$$c(t) - c_0 = \lambda(x(t) + y_c(t)). \tag{2}$$

Here $y_c(t)$ is an unknown function representing the displacement of the corneal reflexion with respect to $x(t)$, while $\lambda$ is a parameter that stands for the fact that, as indicated in [2], the scales on which the corneal and pupil signal move are different. According to Fig.2 in [2] we have $\lambda \sim 1/2$, approximately.

According to the developments in [2], the SMI eye tracker defines the Gaze signal as

$$g(t) = B(p(t) - c(t)) + D, \tag{3}$$

with $B$ and $D$ constants. This is naturally measured in screen pixels, but $B$ and $D$ can be rescaled to get units of angles or any other.

By combining the three equations, we get:

$$g(t) - g0 = B(1-\lambda)x(t) + By(t) - B\lambda y_c(t), \tag{4}$$

with $g0 = B(p_0 - c_0) + D$. Now, we note that the pupil signal can be transformed to the screen pixels coordinates as it is done in [2] to make both signals comparable (see Fig.4 in [2]). We can define $[p(t) - p_0]_{screen} = k(x(t) + y(t))$, with $k$ the transformation constant (equal to the saccade size measured in screen coordinates divided by the saccade size in camera pixels). In order to obtain the same saccade size both for gaze and pupil signals in screen coordinates, we need $B = k/(1-\lambda)$, so that we have

$$g(t) - g0 = kx(t) + \frac{k}{1-\lambda}y(t) - \frac{k\lambda}{1-\lambda}y_c(t). \tag{5}$$

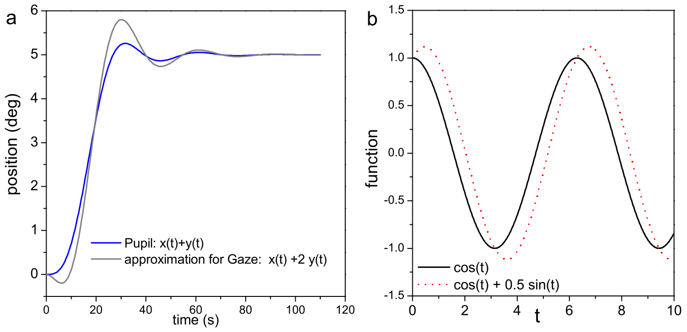


FIG. 1: (Color online) **Approximation for gaze**. a) Example of a 5deg saccade simulated with the model from the main text considering $x(t)+y(t)$ as the pupil signal and $x(t)+2y(t)$ as an approximation for the gaze signal. We see that the curves are in qualitative agreement with those in [2] (see Fig.4 in [2]). Moreover, in this particular example, our approximation for the gaze signal exhibit a backshoot at the begining which is similar to those find in the experiments shown in Fig.9 of [2]. The parameters used in the calculations are $A = 0.03, \mu = 2, \gamma = 0.12, k = 0.45, x_m = 5$. b) Plots of the functions $\cos(t)$ and $\cos(t) + 0.5\sin(t)$ as a sketch of the type of deviance that we expect between the actual PSO of the gaze signal and the PSO of the approximation $x(t) + 2y(t)$.

We can also transform the corneal signal to screen coordinates. To make it compatible with the pupil signal we need a constant $k/\lambda$, so that we have $[c(t) - c_0]_{screen} = k(x(t) + y_c(t))$. The results in the left panels of Fig.4 of [2] strongly suggest that the oscillations of the corneal reflection (with the scaled coordinates used in the figure) are of the same amplitude as the pupil oscillations. This means that we have $y(t) \sim y_c(t)$ (both oscillations of the same amplitude, but not necessarily similar each other in shape). Hence, the third term in the right hand side of Eq. (5) is smaller than the second term (by a factor $\lambda \sim 1/2$), and we can approximate

$$g(t) - g0 \simeq kx(t) + \frac{k}{1-\lambda} y(t) \simeq kx(t) + 2ky(t). \tag{6}$$

Now, redefining $kx(t) \to x(t)$ and $ky(t) \to y(t)$ for the sake of simplicity, and interpreting the results in any coordinate systems, Eq. (6) indicates that, if the pupil dynamics is given by $p(t) - p_0 = x(t) + y(t)$, the gaze dynamics is given approximately by $g(t) - g_0 \simeq x(t) + 2y(t)$. This explains why the PSO of the gaze in Fig. 4 of [2] is an enhanced-amplitude version of the pupil PSO. It can be seen that the positions of the maxima and minima of both signals are almost coincident and so they are the relative amplitudes of the different peaks. (In Ref. [2], the authors indicate "the gaze signal appears an excessive version of the pupil signal".) In Fig. 1.a. of this Supplemental Material, we show calculations using our model that reproduce the type of curves shown in Fig.4 of [2].

The above results indicate that the *qualitative* dependence of the amplitude (and period) of the PSO on the saccade size for the pupil signal should be the same as that for the gaze signal, since both oscillations are essentially determined by the function $y(t)$.

Now, we wonder about the error introduced by neglecting the term $y_c(t)$. Interestingly, results in Fig. 4 in [2] suggest that the corneal reflection PSO have the same period as the pupil PSO, but shifted about a quarter of period in time. This means that the difference or deviation between the approximation $(x(t) + 1/(1-\lambda)y(t))$ and the gaze signal $(x(t) + 1/(1-\lambda)y(t) + y_c(t))$, should be similar to the one existing for instance between the functions $\cos(t)$ and $\cos(t) + 1/2\sin(t)$, which are shown in Fig. 1.b of this Supplemental Material in order to provide a rapid insigth. This deviation is negligible for our qualitative considerations, since although there is an amplitude difference of about 20%, the period is not modified and the temporal shift is quite small (smaller than 1/10 of the period).

* email: bouzat@cab.cnea.gov.ar.

[1] I. Hooge, M. Nyström, T. Cornelissen and K. Holmqvist. Vision Research **112**, 55 (2015).
[2] I. Hooge, K. Holmqvist and M. Nyström, Vision Research **128**, 6 (2016).
